# Supplementary material for: Thermal conductivity of Li$_3$PS$_4$ solid electrolytes with ab initio accuracy
Source: arXiv:2401.12936 ancillary file (2024-06-17)
Supplement: Supplementary file 1 [file Supplemental_Material.pdf]

# Thermal transport of $\text{Li}_3\text{PS}_4$ solid electrolytes with *ab initio* accuracy

## Supplemental Material

Davide Tisi,<sup>1</sup> Federico Grasselli,<sup>1</sup> Lorenzo Gigli,<sup>1</sup> and Michele Ceriotti<sup>1,\*</sup>

<sup>1</sup>*Laboratory of Computational Science and Modeling, Institut des Matériaux,  
École Polytechnique Fédérale de Lausanne, 1015 Lausanne, Switzerland*

(Dated: January 23, 2024)

---

\* michele.ceriotti@epfl.ch

# I. BULK PROPERTIES OF $\text{Li}_3\text{PS}_4$ FROM DFT AND ML-MD

The thermal expansion coefficient is calculated from the ML-MD NpT trajectories using the following expression:

$$\alpha_V = \frac{1}{V} \left( \frac{\partial V}{\partial T} \right) \bigg|_p \quad (\text{S1})$$

where  $V$  is the average volume of the simulation at equilibrium,  $T$  is the temperature and  $p$  is the applied pressure. The derivative w.r.t.  $T$  is computed using finite differences.

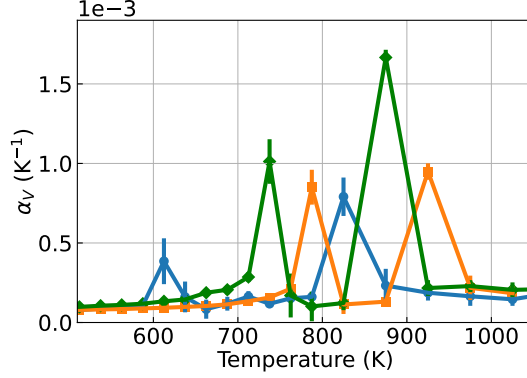

FIG. S1. Thermal expansion coefficient  $\alpha_T$  as a function of the temperature for NpT simulations initialized in the ideal  $\gamma$  structure. Blue line represents the ML-PBESol results, green the ML-PBE0 and orange ML-r<sup>2</sup>SCAN. Error bars obtained through standard block analysis are displayed. The position of the peaks correlates with the phase transition temperatures obtained through the calculation of the heat capacity in Ref. [1].

Another relevant property is the Bulk Modulus which we can extract from the Murnaghan equation of state (MEoS) [2] for the structure at 0 K (see Table S1), and we can compute the temperature-dependent bulk modulus from the volume fluctuations in the NpT MD simulations (see Fig. S2).

| phase    | PBESol [3] | PBESol | r <sup>2</sup> SCAN | PBE0 |
|----------|------------|--------|---------------------|------|
| $\alpha$ | —          | 25.1   | 24.4                | 23.9 |
| $\beta$  | 23.3       | 27.4   | 25.4                | 25.4 |
| $\gamma$ | 32.9       | 37.2   | 40.4                | 39.4 |

TABLE S1. Bulk modulus, in GPa, for the different phases and target functional, obtained from the Murnaghan equation of state (MEoS) computed with the different MLP models. In computing the MEoS, the ionic positions are relaxed for each different volume [4].

While we can compare, with existing literature [3], our predictions for the bulk modulus of  $\beta$  and  $\gamma$  with PBESol model, no available data exists for *ab initio* computations of the bulk modulus at the r<sup>2</sup>SCAN and PBE0 level or for the  $\alpha$  phase.

In Fig. S2 we also show the temperature-dependent bulk modulus  $B(T)$ , obtained via volume fluctuations in NpT:

$$B^{-1} = \frac{1}{k_B T} \frac{\langle V^2 \rangle_{NpT} - \langle V \rangle_{NpT}^2}{\langle V \rangle_{NpT}} \quad (\text{S2})$$

The plots indicate that, by increasing the temperature, the material softens in all phases. The sudden drop of  $B(T)$  at  $T \approx 1000$  K is due to the melting of  $\text{Li}_3\text{PS}_4$ . Furthermore, for simulations initialized in the  $\gamma$  phase, an additional drop of  $B(T)$  at (functional-dependent) critical temperature  $T_c$  indicates the transition to the mixed  $\beta/\alpha$  phase [5].

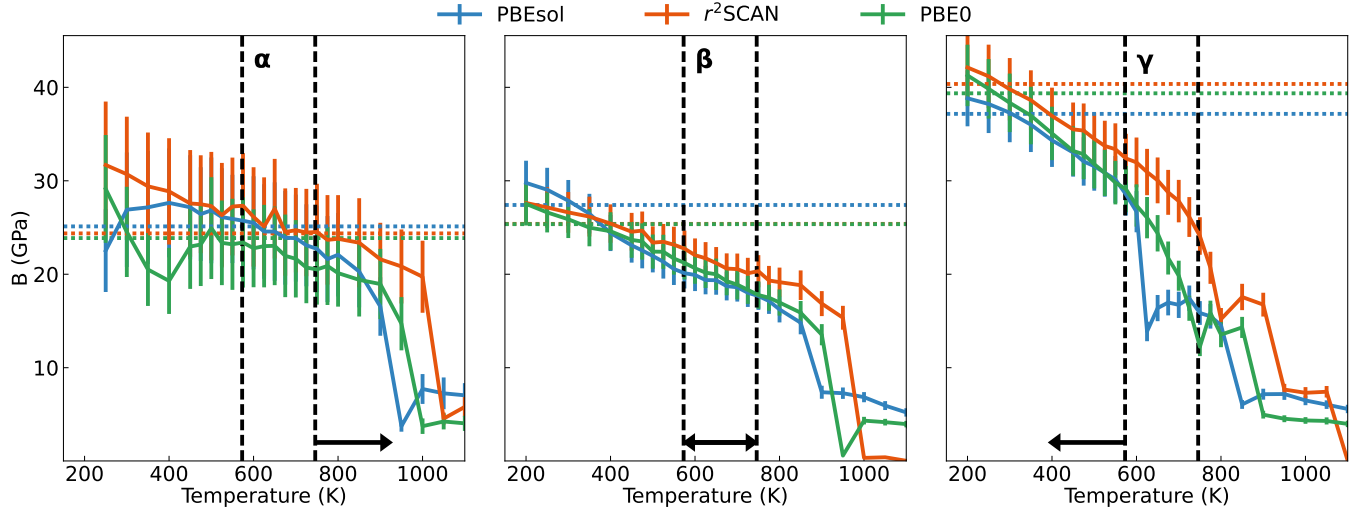

FIG. S2. Bulk modulus  $B$  of the different phases of  $\text{Li}_3\text{PS}_4$  as a function of temperature.  $B$  has been obtained from the volume fluctuations in the NpT MD simulations of Fig. 4 of the main text. The horizontal dotted lines are the values at 0 K obtained in Table S1. The black arrows show the region of experimental stability of a specific phase.

## II. COMPARISON BETWEEN ML AND *AB INITIO* PHONON SPECTRA

Figure S3 shows a comparison between the phonons and the vibrational density of states computed by *ab initio* with the density functional perturbation theory [6] and by the ML-PBESol potential via finite difference. Fig. S4 instead shows a comparison of the phonons and density of states computed by each ML potentials.

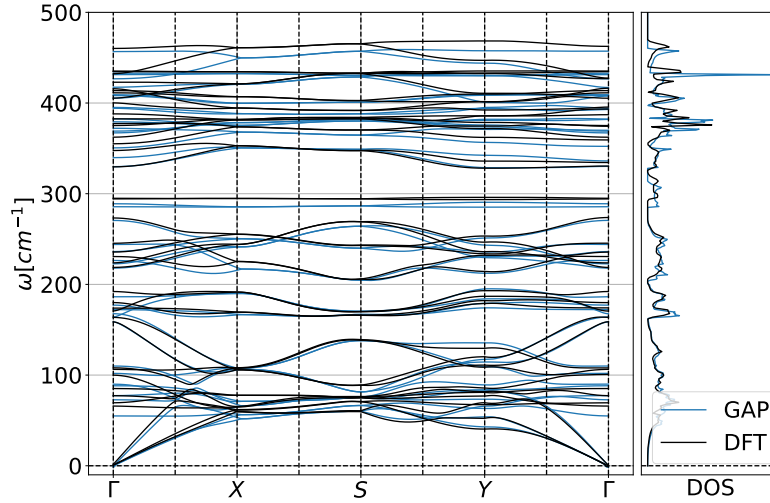

FIG. S3. Phonons and vibrational density of states computed from density functional perturbation theory at the PBEsol level and from finite differences using the ML-PBESol potential.

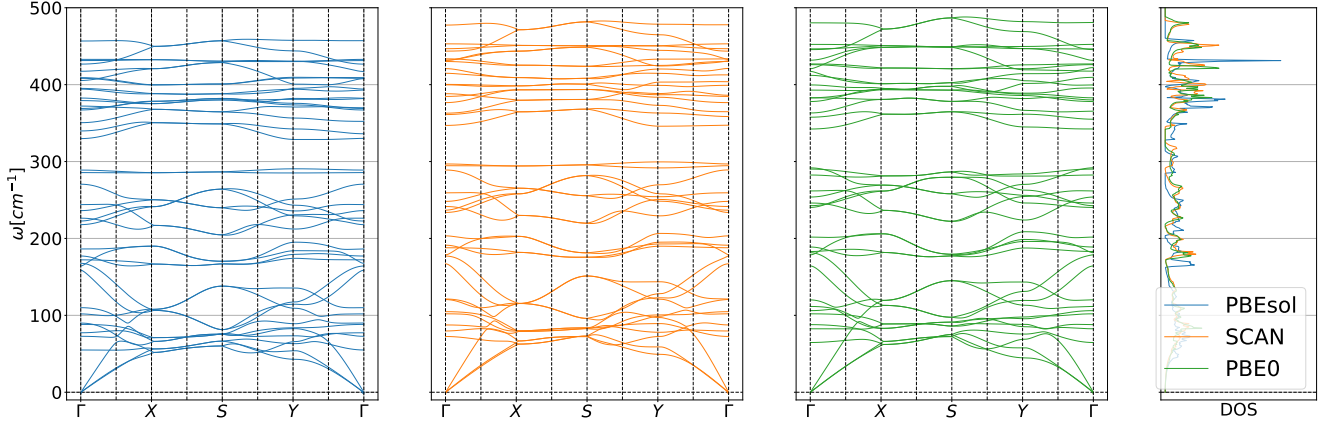

FIG. S4. Phonons and vibrational density of states computed from finite differences using the ML potentials.

### III. THERMAL CONDUCTIVITY OF A COMMITTEE OF MODELS

Figure S5 is the equivalent of Fig. 1 in the main text for a committee of 4 models. As already shown in the main text, even though the models have different distributions of the local energies and, consequently, different energy currents, they all converge to the same value of  $\kappa$ .

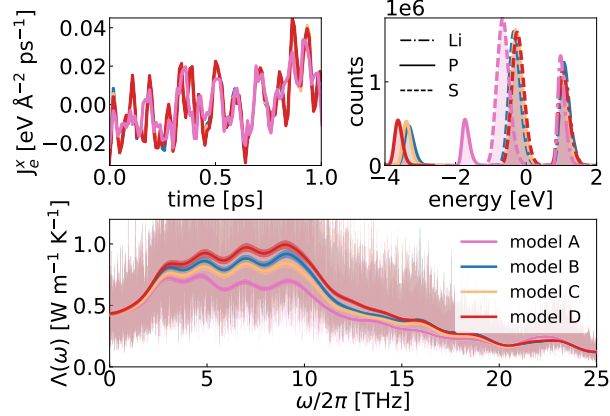

FIG. S5. Non-uniqueness of energy flux and invariance principles of thermal conductivity. (a)  $x$  component of the energy flux  $\mathbf{J}_e$  along a same segment of trajectory (of 200 ps), and (b) distribution of atomic energies per species, computed for the different members of a committee of MLP models. Stars represents the energies of Li, circles of S and diagonal lines the P. (c) Reduced power spectrum and cepstral estimates of  $\kappa$ . All the results are obtained by recomputing the local energies and heat fluxes with the different models on the snapshots of the trajectory generated by the model labeled as A.

Figure S6 shows that the naïve use of  $S_{ee}(\omega)$  instead of  $\Lambda(\omega)$  leads to both wrong and nonsensical results. In fact, not only the values at  $\omega \rightarrow 0$  differs from the correct value of  $\kappa$  (black arrow), taken from Fig. 1 of the main text, but also different ML models give different values of  $S_{ee}(0)$ .

Notice that, from the implementation standpoint, only pair potentials  $v(|\mathbf{r}|)$  prescribe that  $W_{i,\mu\nu} = W_{i,\nu\mu}$ . In fact,

$$\frac{\partial v(|\mathbf{r}_{ij}|)}{\partial r_{i,\nu}} = \frac{\partial v(|\mathbf{r}_{ij}|)}{\partial r_{ji,\nu}} = \frac{1}{|\mathbf{r}_{ji}|} \frac{\partial v(|\mathbf{r}_{ij}|)}{\partial |\mathbf{r}_{ji}|} r_{ji,\nu},$$

where  $\mathbf{r}_{ji} \equiv \mathbf{r}_i - \mathbf{r}_j$ . Hence,  $W_{i,\mu\nu} \propto \sum_j \frac{1}{|\mathbf{r}_{ji}|} r_{ji,\mu} \frac{\partial v(|\mathbf{r}_{ij}|)}{\partial |\mathbf{r}_{ji}|} r_{ji,\nu}$  is invariant under exchange of  $\mu$  and  $\nu$ . In the case of ML potentials with 3-body descriptors, instead, we cannot assume that the atomic virials are symmetric.

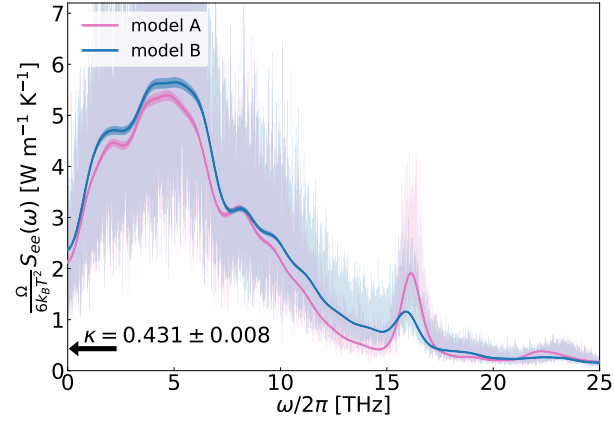

FIG. S6. Effect of incorrect use of  $S_{ee}(\omega)$  instead of the full  $\Lambda(\omega)$ .  $S_{ee}(0)$  not only depends on the ML model, but it is also very different from the correct value, taken from Fig. 1 of the main text and represented by the black arrow.

#### IV. COMPARISON BETWEEN NVT AND NPT RESULTS

The results for  $\kappa$  shown in Fig. 4 in the main text are obtained from NpT simulations. Figure S7 shows that using the barostat does not affect the final result. The blue solid line represents the cepstrum filter for a NpT simulation used in the main text, while the orange line is the filter for a corresponding NVT simulation with a volume equal to the average volume of the NpT one. Both simulations are run for a  $\text{Li}_3\text{PS}_4$  system in the  $\alpha$ -phase at 650 K. The shaded areas represent the true power spectrum. The inset shows the region near  $\omega = 0$  THz.

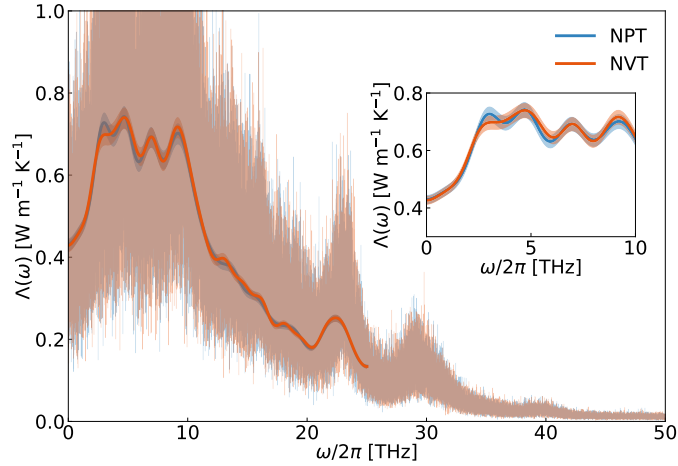

FIG. S7. Power spectrum (shaded areas) and cepstral filter (solid lines) for two simulations of  $\text{Li}_3\text{PS}_4$  in the  $\alpha$ -phase at 650 K. The blue represents an NpT simulation like the one used in Fig. 4 in the main text, while the orange represents a NVT simulation at a volume equal to the average volume of the NpT simulation. The inset represents the region near  $\omega = 0$  THz.

Figure S8 shows the comparison between  $\kappa$  in the  $\gamma$ -phase from NpT simulation (like in Fig. 4 of the main text) and  $\kappa$  from Fig. 3 of the main text from NVT simulations at the volume equal to the one used for lattice methods. This shows that our results are size converged and that the volume equilibration due to thermal expansion has no relevant effects on the results.

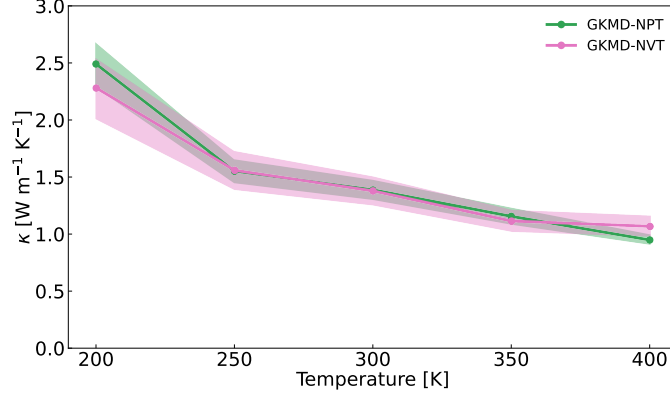

FIG. S8.  $\kappa$  as a function of the temperature, for NpT simulations like in Fig. 4 in the main text and from NVT simulation from Fig. 3. All the simulations are performed with the GAP-PBE0 model.

## V. VOLUME EFFECTS ON THE THERMAL CONDUCTIVITY

In Fig. 4 of the main text we showed that the values of  $\kappa$  depend on the level of theory of the potential. The simulations in Fig. 4 are done in the NpT ensemble, so trajectories at the same temperature but computed with different potentials have different average volumes. To show that the differences in the values of  $\kappa$  are not simply a consequences of the differences in volume, we computed, for the  $\gamma$  at 200 K and  $\alpha$  at 650 K, a NVT trajectory with the ML-PBEsol potential at the average volume of the simulation with the ML-r<sup>2</sup>SCAN potential, and a NVT trajectory with the ML-r<sup>2</sup>SCAN potential at the average volume of the simulation with the ML-PBEsol potential, at the same target temperature. Figure S9 shows that the functional-induced change in equilibrium volume does not significantly affect  $\kappa$ .

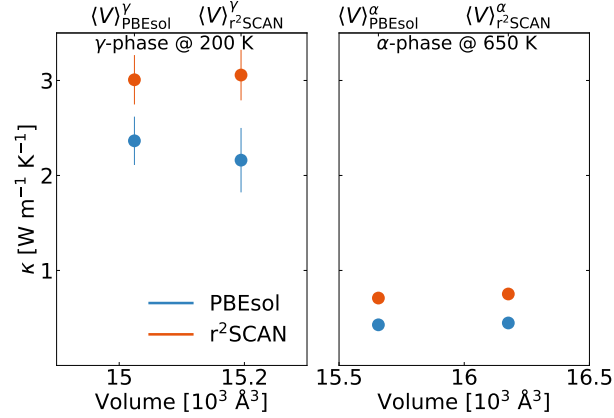

FIG. S9. The figure contains two sets of simulations. We compare the results from Fig. 4 of the main text and the results from an NVT simulation with the ML-PBEsol (ML-r<sup>2</sup>SCAN) potential with the volume fixed to be the average volume of the simulation with the ML-r<sup>2</sup>SCAN (ML-PBEsol) potential in Fig. 4. The left panel contains results for the  $\gamma$  phase at 200 K, the right panel shows results for the  $\alpha$  phase at 650 K.

## VI. LATTICE METHODS

Figure S10 shows the values of  $\kappa$  computed from the lattice methods with quantum occupancy, with different methods and approximations, with and without the interband term. In the figure, QH GK represents the quasi-harmonic Green-Kubo result, which differs from the relaxation-time approximations (RTA) for the inclusion of the interband contribution.  $\kappa_{\text{INV}}$  has been computed with the inversion of the full scattering matrix, while  $\kappa_{\text{FULL}} = \kappa_{\text{INV}} - \kappa_{\text{RTA}} + \kappa_{\text{QH GK}}$ , which corresponds to adding the interband term to the result obtained via the inversion the

scattering matrix.

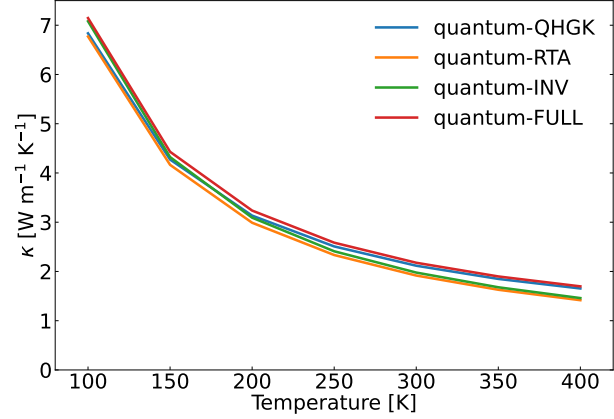

FIG. S10.  $\kappa$  computed with BTE and quantum occupancy, with different methods.

- 
- [1] Lorenzo Gigli, Davide Tisi, Federico Grasselli, and Michele Ceriotti, “Mechanism of charge transport in lithium thiophosphate,” (2023), arXiv:2310.15679 [cond-mat].
  - [2] F. D. Murnaghan, “Finite deformations of an elastic solid,” American Journal of Mathematics **59**, 235–260 (1937).
  - [3] Zhi Deng, Zhenbin Wang, Iek-Heng Chu, Jian Luo, and Shyue Ping Ong, “Elastic properties of alkali superionic conductor electrolytes from first principles calculations,” Journal of The Electrochemical Society **163**, A67 (2015).
  - [4] Giuliana Materzanini, Tommaso Chiarotti, and Nicola Marzari, “Solids that are also liquids: elastic tensors of superionic materials,” npj Computational Materials **9**, 10 (2023).
  - [5] Lorenzo Gigli, Davide Tisi, Federico Grasselli, and Michele Ceriotti, “Mechanism of charge transport in lithium thiophosphate,” arXiv preprint arXiv:2310.15679 (2023).
  - [6] Stefano Baroni, Stefano de Gironcoli, Andrea Dal Corso, and Paolo Giannozzi, “Phonons and related crystal properties from density-functional perturbation theory,” Rev. Mod. Phys. **73**, 515–562 (2001).
